# Supplementary material for: Decentralized Fictitious Play Converges Near a Nash Equilibrium in Near-Potential Games
Source: arXiv:2201.11854 source file (2022-01-27)
Supplement: Supplementary file 1 [file appendix.tex]

% !TEX root = Control of stochastic disease network games via influential individuals.tex

\begin{lemma}\label{col_step2}
 Suppose Assumption \ref{as_finite_eq} holds. The following statements hold:
\begin{enumerate}
    \item There exists $\bar{\alpha}>0$ such that for any $0\le \alpha \le \bar{\alpha}$, the $\epsilon$-NE sets around different equilibrium points, $\Sigma^{(m')}_{\alpha}$ and  $\Sigma^{(m'')}_{\alpha}$ for any $m' \neq m''$  are disjoint,  $\Sigma^{(m')}_{\alpha} \cap \Sigma^{(m'')}_{\alpha}=\emptyset$. 
    \item There exist $\delta>0$ and $\bar{\epsilon}>0$ such that the following inequalities are satisfied,
    \begin{equation}
        N\delta+\bar{\epsilon} < \bar{\alpha},
    \end{equation}
    \begin{equation}\label{eq_bound24}
        q( N\delta+\bar{\epsilon}) < \frac{(\bar{\alpha}- N\delta)d^*}{24NL},
    \end{equation}
\end{enumerate}
 
\end{lemma}

\begin{proof}
\begin{enumerate}

    \item  By Lemma \ref{lem_step1} and Assumption \ref{as_dist_ne}, there exists $\bar{\alpha}$, that satisfies such the condition $q(\bar{\alpha}) \le d^*/4$. Since  $q$ is weakly increasing and, $d^*$ is the minimum distance between any pair of equilibrium points,  for any $\alpha \le \bar{\alpha}$, it follows that $\Sigma^{(j')}_{\alpha} \cap \Sigma^{(j'')}_{\alpha}=\emptyset$.
    
    \item For sufficiently small enough $\delta>0$ by Assumption  \ref{as_dist_ne}, and $\bar{\epsilon}>0$, it holds $N\delta +\epsilon < \alpha$ for any $\epsilon \le \bar{\epsilon}$. Using the fact $\underset{\alpha \rightarrow 0}{\lim}q(\alpha)= 0$  from Lemma \ref{lem_step1}, it gives $q(N\delta +\epsilon)< \frac{\alpha d^*}{48NL} < \frac{(\alpha-N\delta)d^*}{24NL}$.
\end{enumerate}
\end{proof}
